# Supplementary material for: Learning from few examples: Classifying sex from retinal images via deep learning
Source: arXiv:2207.09624 source file (2022-07-20)
Supplement: Supplementary file 1 [file supporting_information.tex]

\section*{Supporting information}

% Include only the SI item label in the paragraph heading. Use the \nameref{label} command to cite SI items in the text.
\paragraph*{S1 Methods.}
\label{S1_methods}
{\bf Detailed description of the methods used for model training and
evaluation.} This section includes further detail on network architecture,
optimization procedure, scoring and dataset augmentation.

\paragraph*{S1 Choice of loss.}
\label{S1_loss} %
{\bf Exploration of loss function structure for training-time validation
  metrics.} This section reveals patterns between the structure of the loss
function and observations of the training-time validation scores.

\paragraph*{S1 Bootstrap method.}
\label{S1_bootstrap_method}
{\bf Details on the bootstrap procedure used.} This section outlines the
bootstrap procedure used to evaluate statistical significance and obtain
confidence intervals.

\paragraph*{S1 Parameter values.}
\label{S1_parameter_values}
{\bf Parameter values used in model training.}  This section contains
information about the parameter values used in model training, specifically
regarding dataset augmentation and parameter governing the optimization
procedure.

\paragraph*{S1 Data statistics.}
\label{S1_data_statistics}
{\bf Statistics for the datasets used in this work.}  Herein is provided the statistics characterizing the datasets used in this work.

%%% Local Variables:
%%% mode: latex
%%% TeX-master: "dlri.tex"
%%% reftex-default-bibliography: ("/Users/aberk/Dropbox/org/bibliography.bib")
%%% End:
